# Supplementary material for: Contextual Data Augmentation for Task-Oriented Dialog Systems
Source: arXiv:2310.10380 source file (2023-10-16)
Supplement: Supplementary file 1 [file appendix.tex]

\section{Parameters}
\label{app:parameters}

In this section we discuss the parameters for our experiment in more details. Our models were implemented in PyTorch. We fine tune BART (base) model for 3 epochs on the dialog augmentation task. We use batch size of $8$, and learning rate $2 \times 10^{-5}.$ We freeze the encoder and embeddings during training. During inference, we use $4$ eval beams. For extrinsic evaluation, we train the Soloist \cite{SOLOIST:PengLLSLG21} model with default hyper-parameters using the original code\footnote{https://github.com/pengbaolin/soloist}. We train the model until the validation loss has decreased for $5$ consecutive evaluations (conducted every $2000$ steps). We train the SG--DST model for $70$ epochs and remaining hyper-parameters set to their default values of the original implementation\footnote{https://github.com/google-research/google-research/tree/master/schema\_guided\_dst}. We select the final model to evaluate on the SGD test set. We train all models using a machine with single V100 GPU. Training BART dialog augmentation model requires approximately $3$ hours, training Soloist model takes approximately $7$ hours, and training SG--DST model takes approximately $26$ hours. 

%\section{Datasets}
%\label{app:datasets}

\section{Metrics} 
\label{app:metrics}

Our evaluation is broken down into two groups of metrics, intrinsic and extrinsic.  Intrinsic metrics attempt to gauge how good the augmentation is with respect to the input, the extrinsic metrics attempt to gauge how well the augmented data is able to improve on some downstream task.

For the intrinsic metrics we compute the following:
\textbf{BLEU} is a lexical, orderless notion of similarity between generated hypothesis text and reference input \cite{papineni-etal-2002-bleu}. This score is computed on ngrams and we track the 1, 2, 3, and 4-gram BLEU scores. We report the average of these 4 BLEU scores as "BLEU".

\textbf{BertScore} is a semantic orderless similarity score. This score is broken into 2 parts, precision and recall. In both scores, each token in the reference (input) and hypothesis (output) sentence is embedded with BERT. BERTScore recall finds for each token in the input, the cosine similarity of the most similar output token, and then averages over these scores. BERTScore Recall finds for each token in the output, the cosine similarity of the most similar input token, then averages over these scores.
BERTScore F1 is the harmonic mean of these two scores above \cite{bertscore-zhang2019}, which we use in our experiments.

\textbf{Bleurt} uses a BERT model fine tuned on synthetically paired sentences from wikipedia (based on existing metrics like BLEU and ROUGE). Then the model is fine tuned on WMT Metrics Task dataset. This gives a supervised notion of sentence similarity taking into account order of tokens and semantics of the sentences (where BLEU and Bert Score only take into account orderless lexical and semantic similarity respectively \cite{bleurt-sellam2020}.

For the extrinsic evaluation on MultiWOZ we use the \textbf{Inform rate} and the \textbf{Success rate} which are the most commonly used metrics on MultiWoZ \cite{SOLOIST:PengLLSLG21}.  
\textbf{Inform rate} is the rate at which the final returned entries from the database are a non-empty subset of the dialog goal’s acceptable entities\cite{Nekvinda2021}. 
\textbf{Success rate} is the rate at which the inform rate condition holds, and the system mentioned all requestable slots required by the user throughout the dialog\cite{Nekvinda2021}.

For extrinsic evaluation on SGD \cite{SGD:RastogiZSGK20} we use the usual metrics {\bf Active intent accuracy}, {\bf Requested slots F1}, {\bf Average goal accuracy}, and {\bf Joint goal accuracy} as defined in \cite{SGD:RastogiZSGK20}.

\section{Additional Experiments}
\label{app:experiments}

In this section we present additional experimental results.

\begin{table}[t]
    \setlength\tabcolsep{3pt}
    \centering
    \scriptsize
    \begin{tabular}{l | l p{1cm} l l}
    \toprule
        \textbf{Models} & \textbf{BLEU} & \textbf{BERT Score} & \textbf{BLEURT} & \textbf{Perplexity} \\ 
        \midrule
        w/ Base BART Augmentation & 0.340 & 0.926 & 0.047 & 114.516 \\ 
        + BS slots & 0.373 & 0.931 & 0.132 & 147.940 \\ 
    \bottomrule
    \end{tabular}
    \caption{\label{table:sgd-ablation-intrinsic}Intrinsic evaluation of the our BART base augmentation model and BS Slot ablation on SGD dataset.}
\end{table}

\subsection{Schema-Guided Dataset(SGD) Results}

We also computed intrinsic metrics on SGD \cite{SGD:RastogiZSGK20} in Table~\ref{table:sgd-ablation-intrinsic}. These results are reasonably consistent with those we find on Multiwoz.  

{\bf Schema Guided Dialog:} The Schema Guided Dialog (SGD) dataset \cite{SGD:RastogiZSGK20}, is a large task-oriented dialog benchmark dataset containing \numprint{22825} dialogs covering $16$ different domains (e.g. Flights, Hotels, Events, Services, Alarm etc.), and split into \numprint{16142} train, \numprint{2482} dev, and \numprint{4201} test dialogs. The dialogs are represented with a flexible and unified schema, which facilitates easier integration of new domain services via zero/few shot dialog state tracking.     

\section{Example Augmented dialogs}

We now present a few example augmentations from our model.  The turn with `*' around them was augmented with the original turn and the augmentation being separated by `::'

\noindent\textbf{Dialog 1:}

In the Table \ref{table:dialog1} we can see that our augmentation of the first turn is very similar to the original even though it was generated without seeing the original turn as input. 

\begin{itemize}
\small
\itemsep0em 
\item{{\em *please put me in touch with the local police, i was just robbed. :: I was robbed and I am looking for help*}}
\item{system: i have information for the parkside police station, is this close to your location?}
\item{user: i don't know, could you just give me the postcode and phone?}
\item{system: the phone number is 01223358966 and the post code is cb11jg.}
\item{user: thank you for your help}
\item{system: you're welcome. the police will help you immediately. goodbye.}
\end{itemize}

We can see that our augmentation of the first turn is very similar to the original even though it was generated without seeing the original turn as input.

\noindent\textbf{Dialog 2:}
\begin{itemize}
\small
\itemsep0em 
\item{user: please see if you can find me a 3-star hotel on the east}
\item{system: i'm sorry we do not have any east hotels that meet your criteria. would you like to try a different part of town?}
\item{user: yes, please look for any 3-star hotel -s in town that include free parking . east is still preferred.}
\item{system: none fits your criteria. can we change the area?}
\item{user: try something in the center of town.}
\item{system: the gonville hotel is an expensive, 3-star hotel in the centre of town. would you like me to book you a room?}
\item{user: yes please . it's for 2 people and 2 nights starting on thursday.}
\item{system: booking was successful.
reference number is : 2v7ewg9e.  is there anything else i can help you with?}
\item{{\em *how about a place to dine in the expensive price range serving indian food. :: I'm also looking for a place to dine that serves indian food*}}
\item{system: i have many. what area would you prefer dining in?}
\item{user: i would like somewhere in the same area as the hotel.}
\item{system: i have 5 all located in the centre}
\item{user: then please pick 1 and give me their phone number band postcode.}
\item{system: saffron brasserie is located at hills road city centre, post code cb21la.  their phone number is 01223354679. can i help with anything else today?}
\item{user: that is everything . thank you for your help.}
\item{system: you are welcome.}
\end{itemize}

This augmentation preserves the user intent and entity ``indian'', but drops the term ``expensive''. In future work, we want to research more into effective ways of leveraging this current turn entity information.

\noindent\textbf{Dialog 3:}
\begin{itemize}
\small
\itemsep0em 
\item{user: can you help me find a train leaving on thursday going to cambridge?}
\item{system: sure, where are you departing from?}
\item{user: departing from broxbourne and leaving after 17:00.}
\item{system: tr1828 is leaving at 17:32, would you like to do that?}
\item{user: yes please . i need reservations for 2 people.}
\item{system: booking was successful, the total fee is 35.79 gbp payable at the station. reference number is : 8br3oq5v.  what else can i assist you with today?}
\item{user: thanks . i am also looking for an expensive place to stay in the north part of town.}
\item{system: unfortunately, i don't happen to have any places that are expensive in the north. can i look for something else for you?}
\item{user: could you please double check to make sure? if that's really the case then try the center}
\item{system: i'm sorry, but the north does not have anything to meet your needs. there are, however, 2 options that meet your needs in the centre. one 3 and one 4 star.}
\item{user: can i get more info on the 3 star one?}
\item{system: sure, gonville hotel is a 3 star rating hotel located at gonville place.  it offers free parking and free wifi.  would you like me to reserve a room?}
\item{{\em *yes, for 4 nights from thursday, and 2 people. :: You're very welcome*}}
\item{system: done! your reference number is v43nqgh7. can i help you with anything else?}

\end{itemize}

Rarely, we generate augmentations like the one above where despite the system/user prompting, it still generates a turn you would expect from the system on a user turn.  This can be alleviated through better prompting and weighting during fine tuning toward the User case.

\subsection{Effects of output filtering}

In our quantitative evaluation, we showed how output filtering based on Bleurt score is crucial in improving the performance of downstream task-oriented dialog systems. To better understand how the filtering chooses turns which are more relevant to the context, we randomly selected few augmentations from the test set and compare the filtered turn to other utterances generated via beam search. Below, we provide two such examples\footnote{We use ellipses to replace some augmentations due to space constraint.}. ``****'' denotes the top ranked utterance by Bleurt. Although we use a large beam size of $25,$ and select top $20$ utterances, we observe that most generated utterances are relevant to the given context. This indicates that in the dialog augmentation task, usually there is a large semantic space of relevant turns between past and future context which makes this problem more challenging. 

\noindent\textbf{Filtering example 1:}

{\em Input turn:}   ``that train is leaving from cambridge on sunday, correct?''

{\em List of augmentations:}

\begin{itemize}
    \item `` I need to go from cambridge to ely''
    
\item ``I need to arrive in Ely by 19:30''
\item ...
\item ``I would like to leave on Sunday''
\item **** ``I need to leave on Sunday from Cambridge'' **** (top ranked by Bleurt score)
\item ``I would like to depart from cambridge''
\item ...
\item ``The train should depart from cambridge''
\item ``I need to arrive by 19:30 in Cambridge''
\end{itemize}

\noindent\textbf{Filtering example 2:}

{\em Input turn:} ``of the 6, what is your restaurant recommendation for good curry?''

{\em List of augmentations:}

\begin{itemize}
    \item ``The restaurant should be in the expensive price range''
\item ***** ``How about one that serves curry food '' ****** (top ranked by Bleurt score)
\item ``The restaurant should be in the expensive price range''
\item ``The restaurant should be in the same area as the restaurant''
\item ``I would like an expensive Indian restaurant in the centre''
\item ...
\item ``I would like one that serves curry food''
\item ...
\end{itemize}
